# Supplementary material for: High extraction efficiency source of photon pairs based on a quantum dot embedded in a broadband micropillar cavity
Source: arXiv:2112.13074 ancillary file (2021-12-24)
Supplement: Supplementary file 1 [file Supplementary_material.pdf]

# Supplementary material: High extraction efficiency source of photon pairs based on a quantum dot embedded in a broadband micropillar cavity

Laia Ginés,[1] Magdalena Moczała-Dusanowska,[2] David Dlaka,[3] Radim Hošák,[4] Junior R. Gonzales-Ureta,[1] Miroslav Ježek,[4] Edmund Harbord,[3] Ruth Oulton,[3] Sven Höfling,[5] Andrew B. Young,[3] Christian Schneider,[6] and Ana Predojević[1,*]

[1]*Department of Physics, Stockholm University, 10691 Stockholm, Sweden*
[2]*Technische Physik, Physikalisches Institut and Würzburg-Dresden Cluster of Excellence ct.qmat, Universität Würzburg, Am Hubland, D-97074 Würzburg, Germany*
[3]*Quantum Engineering Technology Labs, H. H. Wills Physics Laboratory and Department of Electrical and Electronic Engineering, University of Bristol, BS8 1FD, UK*
[4]*Department of Optics, Palacký University, 17. listopadu 12, 77146 Olomouc, Czech Republic*
[5]*Technische Physik, Physikalisches Institut and Würzburg-Dresden Cluster of Excellence ct.qmat, Universität Würzburg, Am Hubland, D-97074 Würzburg, Germany*
[6]*Institut of Physics, University of Oldenburg, D-26129 Oldenburg, Germany*

## DEVICE SIMULATION

Theoretical values of the parameters that characterize the device performance were obtained using FDTD simulations of the pillar structures implemented using Lumerical. A Gaussian broadband dipole source was chosen such that the response to a wide array of frequencies could be recorded. Using a set of 2-D frequency-domain power monitors circumscribed around the micropillar structure in the form of a 6-sided box (as shown in Fig. 1a), we employed the FDTD suite to calculate the power transmission through each monitor plane. Internal efficiency of the device (as plotted in the main text Fig. 2c and Fig. 2d) is estimated as the fraction of power transmitted through the top face of the power monitor box as opposed to the total power generated by the source.

As seen in Fig. 1b, the (un-normalised) top transmission (black line) shows a trend of smooth decay. While the Q factor of the cavity mode remains constant (Q≈285±25) despite changes in the pillar diameter, the mode volume increases. Therefore, the enhancement of the emission into the cavity mode due to Purcell effect decreases and the power transmission through the top face is also weaker as the diameter is increased. On the other hand, the transmission through the sides (red line) experiences periodic peaks and troughs that correspond to diameter values ($D$) such that $D_{trough} = k\frac{\lambda}{n_{GaAs}}$, where $k \in N$, while $D_{peak} = (k-1/2)\frac{\lambda}{n_{GaAs}}$. This behaviour is also reflected in the cavity $\beta$ factor shown in Fig. 1a of the main text, where the probability for the light to be emitted into cavity mode also displays $\frac{\lambda}{n_{GaAs}}$ periodicity. It is expected that the bottom transmission should follow the same trend as the top transmission albeit with a much-reduced transmission due to the asymmetry of the cavity structure. We expect that for a micropillar with a bottom DBR stack large enough the E-field leakage into the substrate should be minimised. However, we observe that despite of 18 bottom DBRs this contribution is still not equal to zero, exhibiting values in the range of 12-25%. We account for this in calculating the minimum/maximum internal efficiency of the pillars (Fig. 2c and 2d) in the main text. Furthermore, we account for the possible discrepancies in the measured vs simulated micropillar diameters by taking an average from an appropriate diameter range ([1.90-2.1]$\mu m$ for the 2.02$\mu m$ pillar in Fig.2c, and [2.65,2.85]$\mu m$ for the 2.75$\mu m$ pillar in Fig. 2d) to produce the range of values plotted in Fig.2a, 2b. The E-field leakage into the substrate can be addresses and minimized, as shown in the Figure 4b of the main text. This can be achieved by having a larger number of the bottom DBRs, or by choosing a substrate with a lower refractive index.

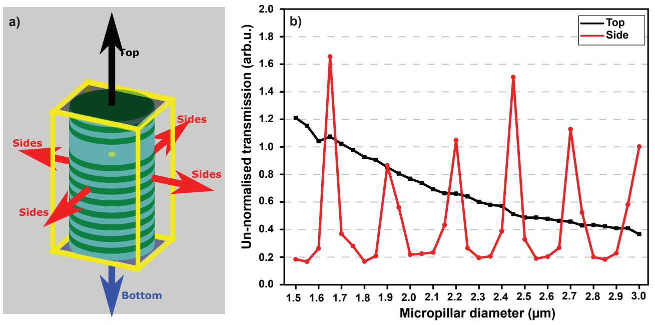


FIG. 1: a) A not-to-scale illustration of the box formed by the 6 two-dimensional power transmission monitors. The box encloses the micropillar structure such that the width of the square bottom and top faces is equal to the pillar diameter, while the height of the box is the height of the pillar itself. The GaAs substrate on which the pillar rests is not pictured in this illustration but is otherwise present in the simulations. b) Power transmission values through the top and the side power monitor box at the resonant frequencies of the cavity mode (910 $nm$) as a function of the pillar diameter.

## PURCELL FACTOR

The emission enhancement values shown in the Fig. 4a of the main text are achieved by using internal functions of the FDTD software that calculate the ratio between the total radiated power by the source and the power the dipole source would radiate in a homogeneous medium. To produce the graph in Fig. 4a, two values were selected for each diameter, such that one is the on-resonant value (i.e. at $\lambda = \lambda_{Cavity}$) and the other is a value extracted at a wavelength far detuned from the cavity resonance (out-of-cavity value).

The emission enhancement values at the wavelength resonant with the cavity mode are shown in green, and the red values correspond to the emission enhancement at a wavelength where there are no modes (cavity or side/lossy modes) present. Spikes in the resonant emission enhancement represent side modes overlapping in wavelength with the cavity mode, which corresponds to higher side losses and lower $\beta$ factors. (see Fig. 1a of the main text). A point of note is that the out-of-cavity values represent Purcell factor of off-resonant light. The values we obtain display a suppression where Purcell factor is below 1. This value indicates that the emission at the wavelengths not resonant to the cavity (and in absence of the side modes) is suppressed. The situation is different on cavity resonance, where the Purcell factor has a value of 1-1.5 (excluding the side modes). This off-cavity suppression combined with the relatively modest on-cavity enhancement help to drastically improve the $\beta$-factor in these low Q pillars.

## DEVICE FABRICATION

The heterostructure we used was grown as a planar cavity with 18 (5) $\lambda/4$ - thick AlAs/GaAs mirror pairs forming the bottom (top) distributed Bragg Reflector (DBR) mirrors. The epitaxial growth of the planar heterostructure are discussed in [1].

Photoluminescence imaging method [2], used to position the micropillars is based on determining the spatial position of a quantum dot with respect to a metallic mask, and simultaneous spectral alignment of the quantum dot emission with respect to the optical resonance of the planar DBR structure. This method provides placement accuracy of <30nm. These steps are achieved in a semi-automatized manner. After selecting a variety of quantum emitters, standard electron beam lithography and reactive ion etching using a Ar/Cl plasma was utilized to define the micropillar around the quantum dots. In the last step, we planarized the sample with benzocyclobuthene to remove the BaF/Cr etch-mask in water without damaging the pillar sidewalls. The final devices, with experimentally determined Q-factor values ranging from 200-300, have diameters between 1.6$\mu m$ and 8$\mu m$. These diameters were chosen to overlap the cavity resonance mode with the quantum dot emission.

## EXPERIMENTAL METHODS

We have implemented Hong-Ou-Mandel measurements using two Michelson interferometers with 3 ns delay. Details of the setup are given in [3].

---

* Electronic address: ana.predojevic@fysik.su.se

[1] S. Maier, et al. Optics Express **22** 8136 (2014).
[2] Y.-M. He et al. Optica **7** 2334 (2017).
[3] L. Gines et al. Optics Express **29** 4174 (2021).
